# Supplementary material for: Spatiotemporal Relationship Reasoning for Pedestrian Intent Prediction
Source: arXiv:2002.08945 source file (2020-02-20)
Supplement: Supplementary file 1 [file Supp.tex]

\documentclass[conference]{IEEEtran}
\IEEEoverridecommandlockouts
% The preceding line is only needed to identify funding in the first footnote. If that is unneeded, please comment it out.
\usepackage{cite}
\usepackage{amsmath,amssymb,amsfonts}
\usepackage{algorithmic}
\usepackage{graphicx}
\usepackage{textcomp}
\usepackage{xcolor}
\usepackage{multirow}
\def\BibTeX{{\rm B\kern-.05em{\sc i\kern-.025em b}\kern-.08em
    T\kern-.1667em\lower.7ex\hbox{E}\kern-.125emX}}

\addtolength{\topmargin}{0.2in}
\usepackage[sort,compress,square,comma,numbers]{natbib}
\PassOptionsToPackage{numbers, compress}{natbib}
\makeatletter
\renewcommand\bibsection%
{
  \section*{\refname
    \@mkboth{\MakeUppercase{\refname}}{\MakeUppercase{\refname}}}
}
\makeatother

\usepackage{sci}
\usepackage{hhline}
\usepackage{caption} 
\captionsetup[table]{skip=5pt}
\usepackage{array}
% Include other packages here, before hyperref.

% If you comment hyperref and then uncomment it, you should delete
% egpaper.aux before re-running latex.  (Or just hit 'q' on the first latex
% run, let it finish, and you should be clear).
\usepackage[pagebackref=true,breaklinks=true,letterpaper=true,colorlinks,bookmarks=false]{hyperref}

\begin{document}

\title{Spatiotemporal Relationship Reasoning \\for Pedestrian Intent Prediction \\ (Supplementary Material) 
% {\footnotesize \textsuperscript{*}Note: Sub-titles are not captured in Xplore and
% should not be used}
%\thanks{Identify applicable funding agency here. If none, delete this.}
}

% \author{\IEEEauthorblockN{Bingbin Liu$^1$, Ehsan Adeli$^1$, Zhangjie Cao$^1$, Kuan-Hui Lee$^2$,} \IEEEauthorblockN{Abhijeet Shenoi$^1$, Adrien Gaidon$^2$, Juan Carlos Niebles$^1$}
% \IEEEauthorblockA{
% \textit{$^1$Department of Computer Science, Stanford University, Stanford, CA 94305, USA}\\\textit{$^2$Toyota Research Institute, Los Altos, CA 94022, USA}\\
% %City, Country \\
% {\texttt \{bingbin, eadeli, caozj, ashenoi, jniebles\}@cs.stanford.edu \quad \{kuan.lee, adrien.gaidon\}@tri.global}}
% \and
% \IEEEauthorblockN{2\textsuperscript{nd} Given Name Surname}
% \IEEEauthorblockA{\textit{dept. name of organization (of Aff.)} \\
% \textit{name of organization (of Aff.)}\\
% City, Country \\
% email address}
% \and
% \IEEEauthorblockN{3\textsuperscript{rd} Given Name Surname}
% \IEEEauthorblockA{\textit{dept. name of organization (of Aff.)} \\
% \textit{name of organization (of Aff.)}\\
% City, Country \\
% email address}
% \and
% \IEEEauthorblockN{4\textsuperscript{th} Given Name Surname}
% \IEEEauthorblockA{\textit{dept. name of organization (of Aff.)} \\
% \textit{name of organization (of Aff.)}\\
% City, Country \\
% email address}
% \and
% \IEEEauthorblockN{5\textsuperscript{th} Given Name Surname}
% \IEEEauthorblockA{\textit{dept. name of organization (of Aff.)} \\
% \textit{name of organization (of Aff.)}\\
% City, Country \\
% email address}
% \and
% \IEEEauthorblockN{6\textsuperscript{th} Given Name Surname}
% \IEEEauthorblockA{\textit{dept. name of organization (of Aff.)} \\
% \textit{name of organization (of Aff.)}\\
% City, Country \\
% email address}
%}

\maketitle

%%%%%%%%% BODY TEXT
\section*{Related Work}
\input{2.related_work.tex}

{%\small
\bibliographystyle{ieeetr}
\bibliography{egbib}
}

\end{document}
